# Supplementary material for: Observation of Spontaneous Ferromagnetism in a Two-Dimensional Electron System
Source: arXiv:2011.01335 ancillary file (2020-11-02)
Supplement: Supplementary file 1 [file SI.2020.ShafayatspinBloch.09.11.pdf]

# Supplementary Information: Observation of Spontaneous Ferromagnetism in a Two-Dimensional Electron System

Md. S. Hossain, M. K. Ma, K. A. Villegas-Rosales, Y. J. Chung,
L. N. Pfeiffer, K. W. West, K. W. Baldwin, and M. Shayegan
*Department of Electrical Engineering, Princeton University, Princeton, New Jersey 08544, USA*
(Dated: November 2, 2020)

## I. EXPERIMENTAL DETAILS

Our material platform is an AlAs quantum well epitaxially grown via molecular beam epitaxy on a GaAs substrate. In particular, our sample contains a 21-nm-wide AlAs quantum well sandwiched by 68-nm-thick $Al_{0.38}Ga_{0.62}$ spacer barriers. Similar to the case of GaAs, as long as the conduction band offset between the barrier and the quantum well is sufficiently large, it is possible to confine carriers in the AlAs quantum well through modulation doping [1–3]. The main difference is that in AlAs the conduction band has lower energy at the X-points of the Brillouin zone instead of the Γ-point. Therefore, the electrons in our AlAs quantum well are confined in the X-point valleys.

In bulk AlAs, electrons occupy three energetically degenerate ellipsoidal (or six half ellipsoidal) conduction band valleys at the six equivalent X-points of the first Brillouin zone [2]. We denote these valleys as [100], [010], and [001] with their major axes lying along the [100], [010], and [001] crystallographic directions, respectively (see Fig. 1*A*). The electrons in each valley possess an anisotropic Fermi surface with longitudinal and transverse effective masses of $m_l = 1.1$ and $m_t = 0.20$ in units of the free electron mass [2].

When an AlAs quantum well is formed along the [001] axis, the confinement in the growth direction splits the three-fold valley degeneracy because of the difference in the effective mass along the in-plane and out-of-plane directions. We refer to the out-of-plane valley as [001], and the in-plane valleys as [100] and [010]. At first sight, one would expect that the [001] valley should be occupied at all well-widths since it has the larger mass along the confinement direction. However, the slightly larger lattice constant of AlAs compared to GaAs causes biaxial compression in the plane of the AlAs layer, lowering the conduction band of the [100] and [010] valleys relative to the [001] valley. This causes the ground-state energies of the two types of valleys to cross at a critical quantum well width of $\simeq$ 6 nm [2]. Above this well-width, the [100] and [010] valleys are occupied; this is the case for our 21-nm-wide AlAs quantum well (Fig. 1*B*).

In the absence of any additional in-plane strain, electrons in our AlAs quantum well occupy two in-plane valleys ([100] and [010]) (Fig. 1*B*). This two-fold valley-degeneracy can be lifted via the application of an in-plane, symmetry-breaking, strain $\Delta\varepsilon = \varepsilon_{[100]} - \varepsilon_{[010]}$, where $\varepsilon_{[100]}$ and $\varepsilon_{[010]}$ are the strain values along [100] and [010] [2]. The valley splitting energy is given by $E_V = \varepsilon E_2$, where $E_2$ is the deformation potential, which in AlAs has a band value of 5.8 eV. Positive strain pushes the energy of the [100] valley up relative to the [010] valley, causing electrons to transfer from [100] to [010], and vice versa for negative strain.

In Fig. 1*C* we show our experimental setup for applying tunable in-plane strain to the two-dimensional electron system (2DES). We glue the sample on one side of a stacked piezoelectric lead-zirconate-titanate actuator with a commercial two-part epoxy [4]. Note in Fig. 1*C* that the sample is glued with its [100] axis along the poling direction of the piezo-actuator. The piezoelectric actuator deforms when a voltage ($V_P$) is applied across its two leads and hence strains the sample glued to its top surface. Thus, we introduce nearly uniaxial, in-plane strain to our 2DES. The strain in our sample is $3.6\times10^{-7}$ per Volt applied to the piezo-actuator.

In order to maintain sufficient strain homogeneity, we used small van der Pauw samples with typical dimensions of 1.5 mm ×1.5 mm. Note that the sample edges are along the GaAs cleave directions, [110] and [$\bar{1}$10] (see Fig. 1*C*). The samples are lapped and polished on the back-side down to 150 $\mu$m in order for the strain to propagate to the 2DES [4]. Electron-beam evaporated Ti-Au alloy on the back-side of the sample shields the 2DES from the electric field generated by the applied $V_P$, and also serves as a back gate which we use to change the 2DES density *in situ*. Electrical contacts to the 2DES are achieved via alloying a eutectic mixture of In and Sn on the corners and the centers of the sample edges at 425 $^o$C for 270 seconds.

Figure 2, which shows the sample's piezo-resistance at a 2DES density $n = 2.90 \times 10^{10}$ cm$^{-2}$ as a function of $V_P$ at zero magnetic field, demonstrates how we tune and monitor the valley occupancy. At $V_P = -310$ V (point **b**), the 2DES exhibits isotropic transport, namely, the resistances measured along the [100] and [010] directions ($R_{[100]}$ and $R_{[010]}$, respectively) are equal, even though the individual valleys are anisotropic. Point **b** corresponds to the case where the [100] and [010] valleys are equally occupied. We refer to this point where the two valleys are degenerate at the "balance" point; for the data shown in Fig. 2, this is achieved via applying a piezo bias of -310 V which we refer to as $V_b$.

For $\Delta\varepsilon > 0$, as electrons transfer from [100] valley to [010] valley, $R_{[100]}$ decreases (black trace in Fig. 2) because the electrons in [010] valley have a small effective mass and therefore higher mobility along [100] [2]. (Note that the total 2DES density remains fixed as strain is applied.) The resistance eventually saturates (point **c**), when all electrons are in the [010] valley [2, 5, 6]. For $\Delta\varepsilon < 0$, $R_{[100]}$ increases and eventually saturates (e.g., point **a**), as the electrons are transferred to [100] valley which has a large mass and a low mobility along [100]. As expected, the behavior of $R_{[010]}$ is opposite to that of $R_{[100]}$.

In our measurements, except for the data presented in Section III below, we use $\Delta\varepsilon > 1\times10^{-4}$, so that only the [010] valley is occupied. For data shown in Section III, we bias $V_P$ so that either the two valleys are degenerate (Section III.A), or the electrons are divided unequally between the two valleys (Section III.B). To achieve this partial occupancy, we assume that the valley occupations are linearly proportional to the strain applied relative to the balance point [2]. For example, point **d** in Fig. 2 corresponds to 75% of electrons occupying valley [100] and 25% valley [010]. Conversely, at point **e**, 25% of electrons occupy valley [100] and 75% occupy valley [010]. Furthermore, to obtain the data for [100] valley occupancy, presented in Section III.B, we use $\Delta\varepsilon < -1\times10^{-4}$, so that all the electrons occupy the [100] valley.

It is worthwhile noting that, a finite $V_P$ is required to attain a balance point (point **b**) in our experiments [2, 5, 7]. For example, for the data shown in Fig. 2, $V_b$ is equal to $-310$ V. Such offset in the balance point occurs because of the cooldown- and sample-dependent residual strain originating from the difference in thermal contraction coefficients of the sample, glue and the piezo-actuator during the cooling process [2, 5, 7].

We carried out our experiments in a $^3$He cryostat with a base temperature of $T \simeq 0.30$ K. We use the back gate to tune the 2DES density $n$, which we describe in units of $10^{10}$ cm$^{-2}$ throughout the manuscript and the Supplementary Information.

In Fig. 3 we demonstrate our measurement setup, showing the voltage and current leads. We use two lock-in amplifiers, one for measuring the voltage ($V_{AC}$) across the sample and another to measure the current ($I_{AC}$) passing through the sample. Resistance is then determined from $V_{AC}/I_{AC}$ via passing a small (1 nA) AC excitation of frequencies 3.0 Hz (for $n > 1.80$) and 1.7 Hz (for $n \leq 1.80$). Note that a direct measurement of current is necessary, especially for low densities when the values of resistance are very large. Since the lock-in amplifier has a finite input impedance, which is about 10 M$\Omega$ for our setup, it causes a portion of the current to flow through the lock-in amplifier to the ground instead of passing through the sample. Therefore, one has to measure the current that flows through the sample directly to obtain an accurate measure of resistance.

## II. RESISTANCE VS. $B_{||}$ NEAR THE METAL-INSULATOR TRANSITION

As shown in Fig. 3*A* of the main text, we observe a change from metallic to insulating transport at a density $n \simeq 3.2$. In this Section, we discuss magnetotransport data as a function of the parallel magnetic field $B_{||}$ near this metal-insulator transition (MIT).

In Fig. 4, we show $R_{[100]}$ vs. $B_{||}$ data, similar to the data in Fig. 1*C* of the main text, including here the traces for a few more densities near the MIT. As we lower the 2DES density, starting from $n \simeq 3.60$, we observe a glimpse of an additional feature at very low $B_{||}$, marked with blue arrows in Fig. 4. It becomes more prominent as we approach the MIT at $n \simeq 3.20$. The additional feature is manifested by a sudden rise in magnetoresistance slope at very low $B_{||}$. The slope abruptly decreases above a certain magnetic field (marked by the blue arrows in Fig. 4), and $R_{[100]}$ increases nearly linearly with $B_{||}$, eventually saturating once $B_{||} = B_M$ is reached (see red arrows in Fig. 4). This feature at a very small $B_{||}$ may imply another transition besides the spin transition at $B_M$. While we do not know its origin, it is very intriguing that this feature only exists in a narrow density range near the MIT ($n \simeq 3.2$). We surmise that there might be a correlation between the appearance of the feature and the MIT.

## III. ROLE OF THE VALLEY DEGREE OF FREEDOM IN THE SPIN POLARIZATION OF THE 2D ELECTRON SYSTEM

In the main text, we mostly focused on the spin polarization when only one valley is occupied and briefly discussed the ferromagnetic transition as a function of valley occupancy. In this Section, we elaborate on the spin polarization of our 2DES when the electrons occupy two in-plane valleys, [100] and [010].

### III. A. Comparison Between Valley-Polarized and Valley-Degenerate 2D Electron System

This subsection delineates a comparative study of the spin polarization and the ferromagnetic transition between the valley polarized (e.g., point **c** in Fig. 2) and valley degenerate (e.g., point **b** in Fig. 2) 2DESs.

In Figs. 4*A*-*C* of the main text, we presented the spin polarization of a valley degenerate 2DES. Here, in Fig. 5 we show $B_M$ and spin susceptibility data for the single-valley and valley-degenerate cases together in the same plot. It is clear from Fig. 5 that the critical density for the ferromagnetic transition in a valley-degenerate 2DES ($n_{c(2V)}$) is smaller than that of a single-valley 2DES ($n_{c(1V)}$). This finding of smaller critical density for

full magnetization in a valley-degenerate 2DES is consistent with previous measurements [8–10] and theoretical calculations [11] concluding that the enhancement of the spin susceptibility, at a given density, is smaller for a two-valley system compared to a single-valley one. A possible way to understand this phenomenon is that the additional valley degree of freedom modifies the inter-valley exchange interaction, which also influences the spin exchange interaction, and leads to a change in the onset density of the spontaneous ferromagnetism.

### III.B. Spin Polarization of the 2D Electron System with Unequally Occupied Valleys

As seen in Section III.A, the valley-degenerate 2DES requires a smaller density than the single-valley 2DES to exhibit the ferromagnetic transition. In this subsection, we elaborate on the evolution of $B_M$ as we tune the valley occupancy, from a single-valley case to a valley-degenerate case. How we achieve this partial valley occupancy is discussed in Section I (Fig. 2).

In Figs. 6*A*-*E*, we plot resistance vs. $B_{||}$ data as a function of valley occupancy, taken at five different densities. It is clear for all the densities that the magnetic field required to magnetize the system, i.e. $B_M$, is the largest when the valleys are degenerate. As we lift the degeneracy and move towards valley polarization, $B_M$ starts to drop and eventually attains its smallest value when the electrons are completely valley polarized. This is again true for all the densities, as seen in Figs. 6*A*-*E* and summarized in Fig. 6*F*. This means that the spin susceptibility is maximum when the 2DES is valley-polarized and minimum when the valleys are degenerate, for a given density. Thanks to this interplay between the spin and valley degrees of freedom, it is possible to control the onset of the ferromagnetic transition via tuning the valley occupancy.

## IV. COMPARING THE RESISTANCE VALUES AT ZERO AND ABOVE MAGNETIZING FIELD NEAR THE SPIN POLARIZATION TRANSITION

Here we address an important question: At $n_c = 2.00$, where the 2DES makes a transition to a fully-spin-polarized state, what is the value of its resistance, and how does this value compare with the resistance at slightly higher densities (just above the transition), say, at $n = 2.10$? More importantly, is the resistance value at $n_c = 2.00$, which is constant and independent of $B_{||}$, close to the saturation value of the resistance at $n = 2.10$ at high $B_{||}$, above $B_M$? A positive answer would be consistent with our conjecture that the 2DES is fully spin polarized at $n = 2.00$ without the application of any magnetic field.

To address this point, we show in Fig. 7 resistance ($R_{[100]}$) values at $B_{||} = 0$ and 3 T as a function of density. In the density range of Fig. 7 data, the 2DES becomes fully spin polarized once $B_{||}$ reaches 3 T (see Fig. 1*C*). We find that $R_{[100]}$ at 3 T (green data points) is larger than its value at $B_{||} = 0$ T (blue data points) by about a factor of two. As the density is lowered to $n_c = 2.00$, $R_{[100]}$ becomes independent of $B_{||}$. Importantly, it is clear in Fig. 7 that the value of $R_{[100]}$ at $n_c = 2.00$ is close to the saturated value of $R_{[100]}$ at $B_{||} = 3$ T at $n = 2.10$. Furthermore, as discussed in the main text, near the full spin polarization transition, there is hysteresis in $R_{[100]}$ vs. $B_{||}$ when the magnetic field sweep direction is reversed. The hysteresis leads to a shift in the minimum polarization, i.e. minimum resistance, to a finite $B_{||}$; see the inset to Fig. 7. In Fig. 7 we also show the resistance values at the $R_{[100]}$ minima using open symbols. These points further elucidate the large increase in resistance at $B = 0$ from $n = 2.10$ to 2.00. This observation indicates that the resistance approaches the expected high field value at $n_c = 2.00$, rather than staying near the value expected for an unpolarized 2DES at $n \geq 2.10$. This is consistent with our conclusion that the 2DES is fully spin polarized at $n_c = 2.00$ at $B_{||} = 0$, just as it is at $n = 2.10$ at $B_{||} = 3$ T.

For the case where the electrons occupy two valleys, the evolution of $R_{[100]}$ as a function of density also corroborates our conclusion of full spin polarization when $R_{[100]}$ becomes independent of $B_{||}$. Figure 8 captures $R_{[100]}$ values at $B_{||} = 0$ and 3 T as a function of density. Similar to Fig. 7, here green and blue data points denote the resistance values at $B_{||} = 0$ and 3 T, respectively; see Fig. 4*A* of the main text for $R_{[100]}$ vs. $B_{||}$ traces. At $n = 1.40$, where $B_M$ vanishes, the value of $R_{[100]}$ at $B = 0$ is close to the high-field value of $R_{[100]}$ at $n = 1.50$. This trend strengthens our conclusion that the valley-degenerate 2DES is fully spin polarized at $n = 1.40$ at $B_{||} = 0$, and the validity of associating $B_{||}$-independence of resistance to ferromagnetism.

## V. MEASUREMENTS OF DIFFERENTIAL RESISTANCE AS A FUNCTION OF DC BIAS

Measurements of sample response as a function of applied DC bias provide information on the *I*-*V* characteristics of the sample. We use such measurements to probe the pinned Wigner solid phase as shown in Fig. 3*B* of the main text. For these measurements, we use a setup shown in Fig. 9. The DC input is taken from the lock-in amplifier and the DC current that flows through the sample is obtained via measuring the voltage drop across a known series resistance (1 kΩ) using a high-precision DC voltmeter. On the other hand, a small AC signal (0.5 nA, 1.7 Hz) is used to extract the differential resistance directly from the lock-in amplifier. Note that, to measure

$V_{AC}$ and $I_{AC}$, a scheme similar to Fig. 3 is used where we measure $I_{AC}$ using a separate lock-in amplifier; this enables us to measure large values of differential resistances ($dV/dI$) (see Fig. 10).

## VI. DENSITY DEPENDENCE OF THE PINNED WIGNER SOLID

In Fig. 3*B* of the main text, we showed the density dependence of $dV/dI$ as a function of applied DC bias current, taken at different densities. The data show the onset density for the non-linear *I*-*V* characteristic, which we interpret to signal the formation of a pinned Wigner solid. In this Section, we elaborate on the density dependence of the voltage bias threshold of the non-linear $dV/dI$.

By performing integration over our $dV/dI$ vs. $I_{DC}$ data, we can obtain the voltage drop along the direction of the current passing through the sample. In Figs. 10*A*, *B*, we plot this voltage drop as a function of $I_{DC}$. The plots exhibit a vanishing non-linearity as the density is raised to $n > 1.70$.

It turns out that presenting our $dV/dI$ data as a function of the voltage drop reveals important information. Figures 10*C*, *D* show such data. As seen in Figs. 10*C*, *D*, $dV/dI$ decreases rather sharply above a certain threshold voltage, i.e. electric field; that is required to depin the Wigner solid. Intriguingly, this threshold voltage depends strongly on the electron density. At very low densities, this depinning voltage is very large. However, it drops quite abruptly as we raise the density (Fig. 10*D*). And, similar to the $dV/dI$ vs. $I_{DC}$ data in Fig. 3*B*, $dV/dI$ vs. $V$ traces become linear and nearly flat above $n = 1.70$ (Fig. 10*D*), the density which we associate with the transition between a liquid and a pinned Wigner solid.

## VII. TEMPERATURE DEPENDENCE OF THE NON-LINEAR *I*-*V* AND THE MELTING OF THE WIGNER SOLID

In this Section, we elaborate on the temperature dependence of $dV/dI$ as a function of electron density. We interpret the disappearance of the non-linear DC response above a critical temperature $T_c$ to signal the thermal melting of the Wigner solid.

We show in Fig. 11 $dV/dI$ data as a function of temperature for five different densities. As seen in Fig. 11*A*, $T_c$ at $n = 1.20$ appears to be between 0.95 K and 1.00 K. As we raise the density, $T_c$ seems to decrease slightly. For example, at $n = 1.50$, the non-linearity disappears at $T = 0.92$ K. As we further raise the density and approach the density ($n = 1.80$) above which the Wigner solid disappears (signaled from the disappearance of the non-linear *I*-*V*), $T_c$ drops rapidly (see Fig. 11*E*). For instance, at $n = 1.70$, the non-linearity in the $dV/dI$ data disappears between $T = 0.42$ K and 0.48 K (Fig. 11*E*), much lower than the range 0.81 to 0.92 K where the non-linearity disappears at $n = 1.50$ (Fig. 11).

## VIII. APPLICABILITY OF THE MERMIN WAGNER THEOREM?

In a seminal paper in 1966, Mermin and Wagner (MW) theoretically showed that, at any non-zero temperature, there can be no ferromagnetism in one or two dimensions [12]. The model MW use is the isotropic Heisenberg spin system with finite-range exchange interaction, and their conclusion is based on theoretically demonstrating that spin-fluctuations destabilize ferromagnetic (as well as anti-ferromagnetic) order in an infinitely-large 2D system. We would like to note that the MW theorem might not be directly applicable to our experiments because:

(*i*) Our sample has a finite size (about 1.5 mm by 1.5 mm).

(*ii*) The 2DES in our sample has a finite (non-zero) electron layer thickness; this may help stabilize the ferromagnetic order.

(*iii*) The 2D electrons in our AlAs sample occupy a valley with an anisotropic effective mass. Electron-electron interaction in an anisotropic system is different from an isotropic system, possibly allowing a violation of the MW theorem.

## IX. RELATED SYSTEMS/PHENOMENA

As discussed in the main text, spin-polarization and metal-insulator transition in dilute 2D carrier systems have been subjects of great interest. However, as described in the main text, prior to our work described here, there have been no clear reports of itinerant ferromagnetism in a system of electrons in the limit of zero magnetic field. In this Section, we discuss several plausible candidates that might exhibit such a phenomenon. We also briefly discuss the investigations on spontaneous magnetization in two exotic systems.

### IX.A. Spin Polarization of 2D Electrons in Other Semiconductor Systems

A large $r_s$ that is required to observe a full magnetization can possibly be obtained in other 2D systems. One such candidate for the experimental realization of spontaneous ferromagnetism is the 2DES at the MgZnO/ZnO interface [13, 14]. Similar to our AlAs quantum wells, this system also hosts a large-mass, high-quality 2DES

[13, 14], and can potentially be a platform to exhibit a ferromagnetic transition at zero magnetic field.

Another emerging material platform is the 2DES in a monolayer of $MoS_2$. In the $MoS_2$ 2DES, $r_s$ is large thanks to the large electron effective mass and small dielectric constant. However, $MoS_2$ has a complex energy band structure: the 2D electrons occupy multiple conduction-band valleys, and also there is a strong spin-orbit interaction, linking the spin and valley degrees of freedom [15]. (This is very different from our AlAs 2DES where we can control the spin and valley degrees of freedom individually because there is no spin-valley locking or spin-orbit interaction.) Recent studies by Roch *et al.* [15, 16] report the observation of spin-polarized electrons at electron densities $n \simeq 5 \times 10^{12}$ cm$^{-2}$, which correspond to $r_s \simeq 5$. A subsequent theoretical work [17] supports such a ferromagnetic phase. In this theory, the ferromagnetism arises from non-analyticities which go beyond Fermi liquid theory. Note that the data in Refs. [15, 16] were taken in a very large magnetic field (9.0 T). It is also worth noting that magnetotransport data in nominally similar samples at comparable densities and magnetic fields [18] exhibit Shubnikov-de Haas oscillations which do not appear to be consistent with a fully-polarized system.

### IX.B. Ferromagnetism in Exotic Fermionic Systems

Itinerant ferromagnetism has been observed in three-dimensional systems [19, 20]. However, these observations were made in ultra-cold atoms, not in a system of electrons.

There is also a very recent study demonstrating an interaction-driven spin polarization of composite fermions [21]. Composite fermions are quasiparticles formed in finite magnetic fields, at and near the half-filling of the lowest Landau level. Experiments performed in a GaAs 2DES show that the composite fermions are fully spin polarized at high electron densities thanks to a large Zeeman energy. However, as the density is lowered, the composite fermions lose their full magnetization and become partially spin polarized. This is expected and stems from a relative reduction of the Zeeman energy compared to the Coulomb energy [22]. Surprisingly, however, as the density is further reduced, composite fermions make a sudden transition back to a fully-magnetized state. This spontaneous magnetization of composite fermions is reminiscent of the Bloch ferromagnetism. Moreover, the theoretical calculations based on quantum Monte Carlo analysis presented in Ref. [21] suggest that the full magnetization of the composite fermions at very low densities occurs because of an enhanced interaction between composite fermions due to Landau level mixing, which is significant at small $n$. It is worth emphasizing that, while the interaction-driven spin polarization is thus seen in composite fermion quasiparticles formed in a finite perpendicular magnetic field, spontaneous ferromagnetism for electrons at *zero magnetic field*, has remained elusive prior to our work on AlAs 2DES presented in this manuscript.

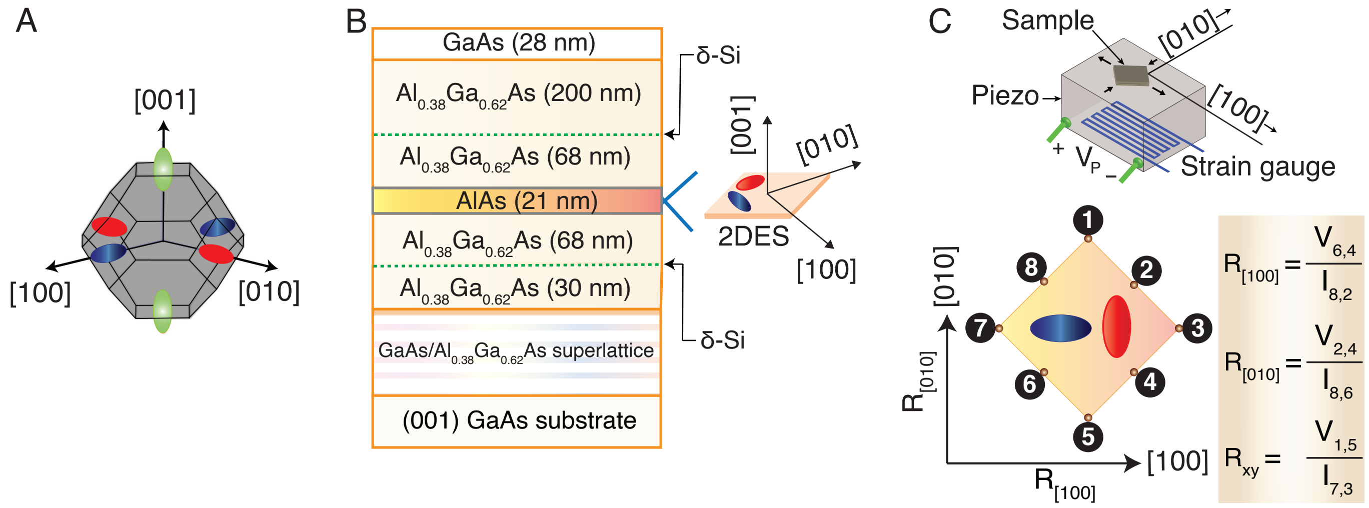


FIG. 1. ($A$) First Brillouin zone and constant energy surfaces of the lowest-energy bands for bulk AlAs, showing the [100], [010], and [001] valleys; [100], [010], and [001] refer to the crystallographic directions. ($B$) Structure of our AlAs 2DES grown on a GaAs substrate. The growth direction is [001]. The AlAs layer is under compressive biaxial strain because of the slightly larger lattice constant of AlAs relative to GaAs. This strain results in the occupancy of [100] and [010] valleys only. ($C$) Schematic of the experimental setup for applying in-plane strain ($\Delta\varepsilon$). The sample is glued on top of a piezo-actuator, and strain is introduced when a bias voltage ($V_P$) is applied to the actuator's leads. The sample geometry, including the orientation of the two occupied valleys ([100] and [010]), are also shown. Contacts to the sample are denoted by 1-8. For $R_{[100]}$, we pass current from contact 8 to 2 and measure the voltage between contacts 6 and 4. For $R_{[010]}$, the current is passed from contact 8 to 6 and we measure the voltage between contacts 2 and 4. On the other hand, for $R_{xy}$, we pass current from contact 7 to 3 and measure the voltage across contacts 1 and 5.

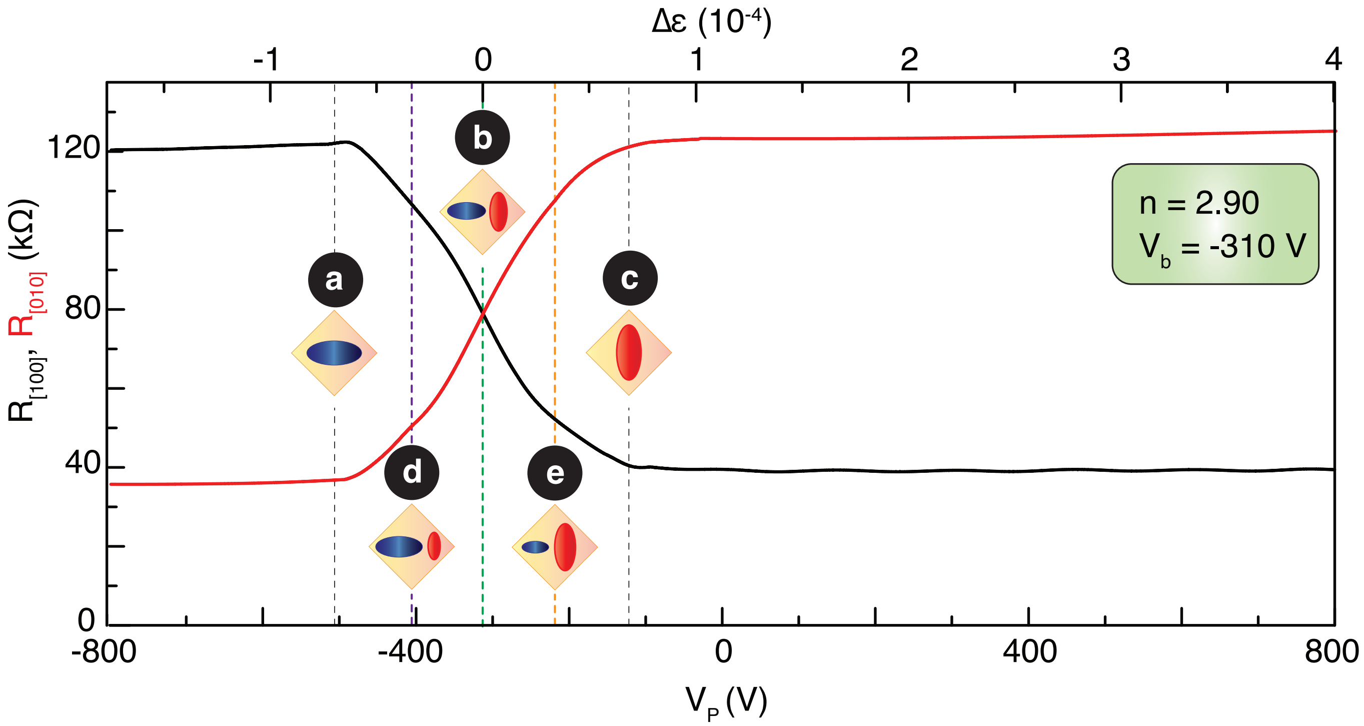


FIG. 2. Piezo-resistance of the sample at a density $n = 2.90 \times 10^{10}$ cm$^{-2}$ as a function of piezo bias $V_P$ and in-plane strain $\Delta\varepsilon$ (top axis). Points **a** - **e** mark the valley occupation. The "balance" point, where the two ([100] and [010]) valleys are equally occupied, is achieved at a piezo bias of $V_b = -310$ V. We can attain different valley occupancies by controlling $V_P$, i.e. $\Delta\varepsilon$.

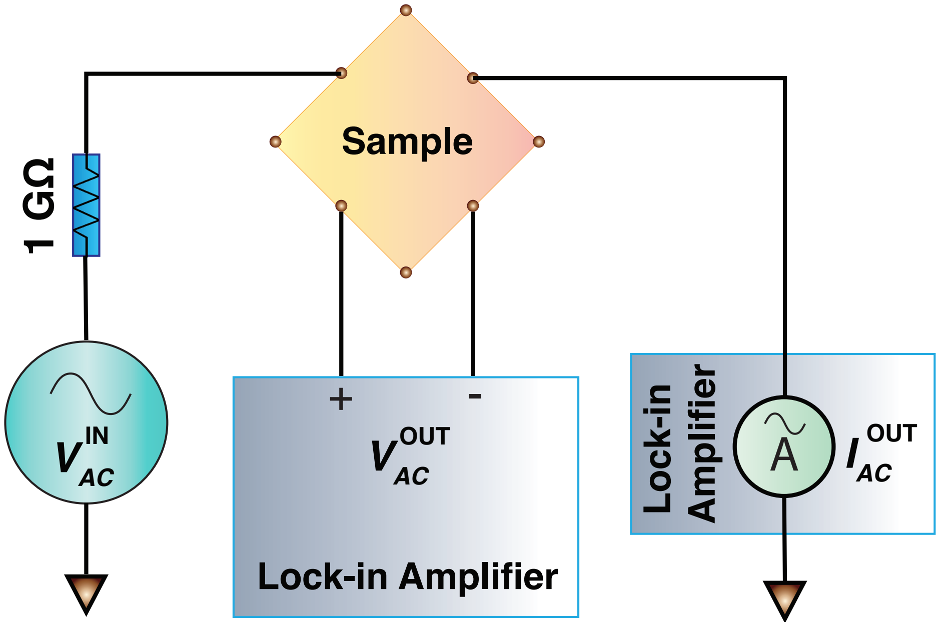


FIG. 3. Experimental setup showing the current injection and voltage probes used to measure $V_{AC}$ and $I_{AC}$ in order to obtain the sample resistance.

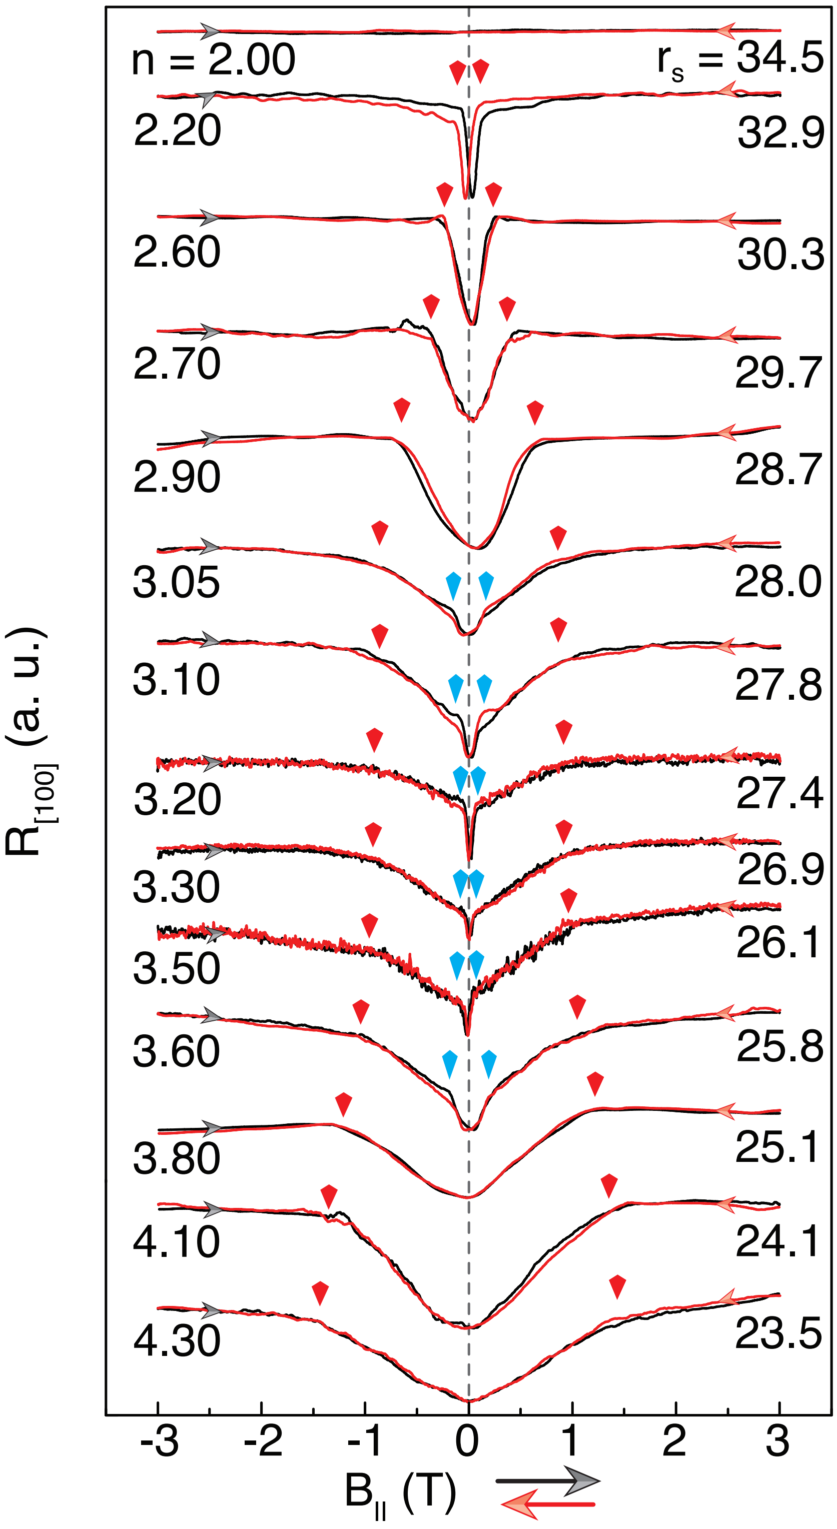


FIG. 4. $R_{[100]}$ vs. $B_{||}$ data taken at different 2DES densities. Traces are shown for both up- and down-sweeps of $B_{||}$, and are offset vertically for clarity. The vertical red arrows mark the positions of $B_M$ above which the resistance saturates. In all the traces, the saturated value of magnetoresistance is almost twice the resistance at $B = 0$. In the density range $3.0 \lesssim n \lesssim 3.6$, the traces exhibit an additional feature at a very small $B_{||}$ (marked with blue vertical arrows). When the 2DES density is tuned away from this density range, the extra feature disappears.

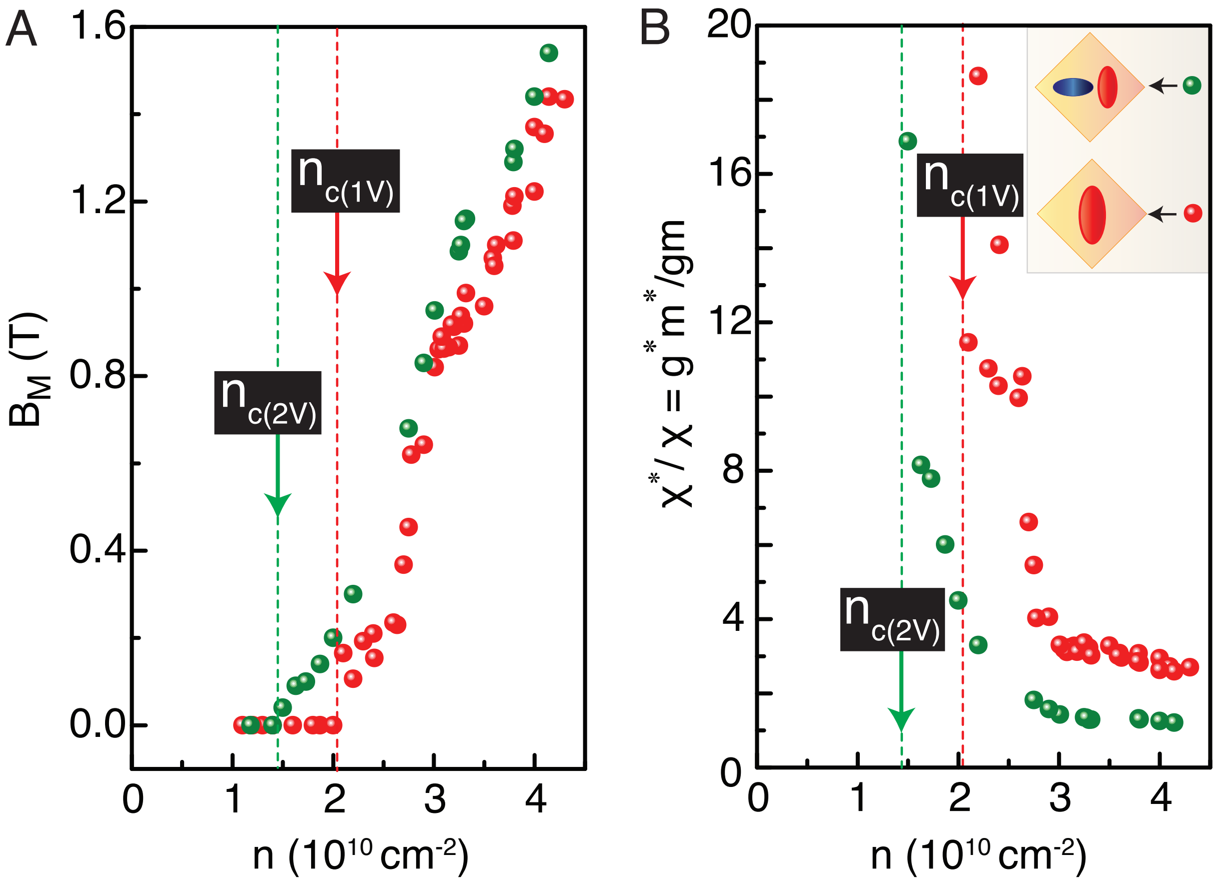


FIG. 5. Comparison of $B_M$ and spin susceptibility for the single-valley and valley-degenerate 2DESs, highlighting the difference in the critical density below which the system makes a ferromagnetic transition.

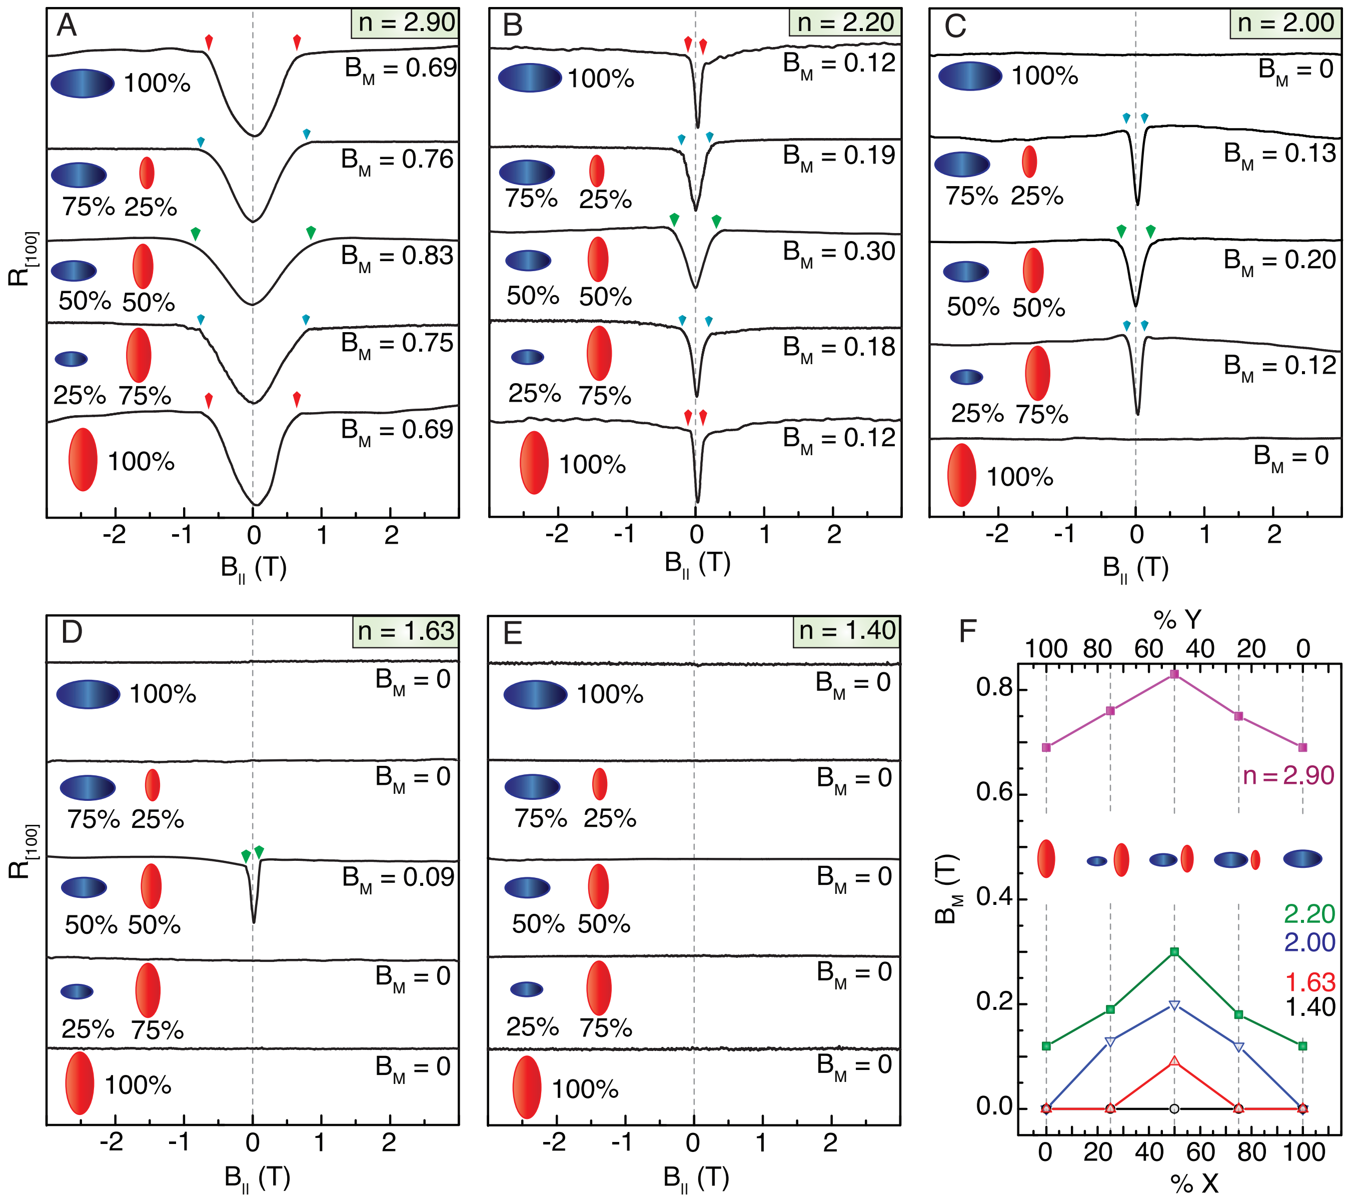


FIG. 6. Evolution of $B_M$ as a function of valley occupancy. (*A-E*) Resistance vs. parallel magnetic field data taken at $T = 0.30$ K for different 2DES densities demonstrating the effect of the valley occupancy on $B_M$. Traces are offset vertically. For each trace, the measured value of $B_M$ is indicated (in units of T). At a fixed density, the 2DES has the smallest $B_M$ when only one valley (either [100] or [010]) is occupied. As electrons start transferring from one valley to the other, $B_M$ increases and reaches its maximum value when the valleys are equally occupied. The single-valley case reaches the ferromagnetic transition at the largest density while the valley-degenerate case requires the smallest density. (*F*) $B_M$ plotted against the valley occupancy, summarizing the data in (*A-E*), and showing a clear increase in $B_M$ as we move from a single-valley case towards the valley-degenerate case.

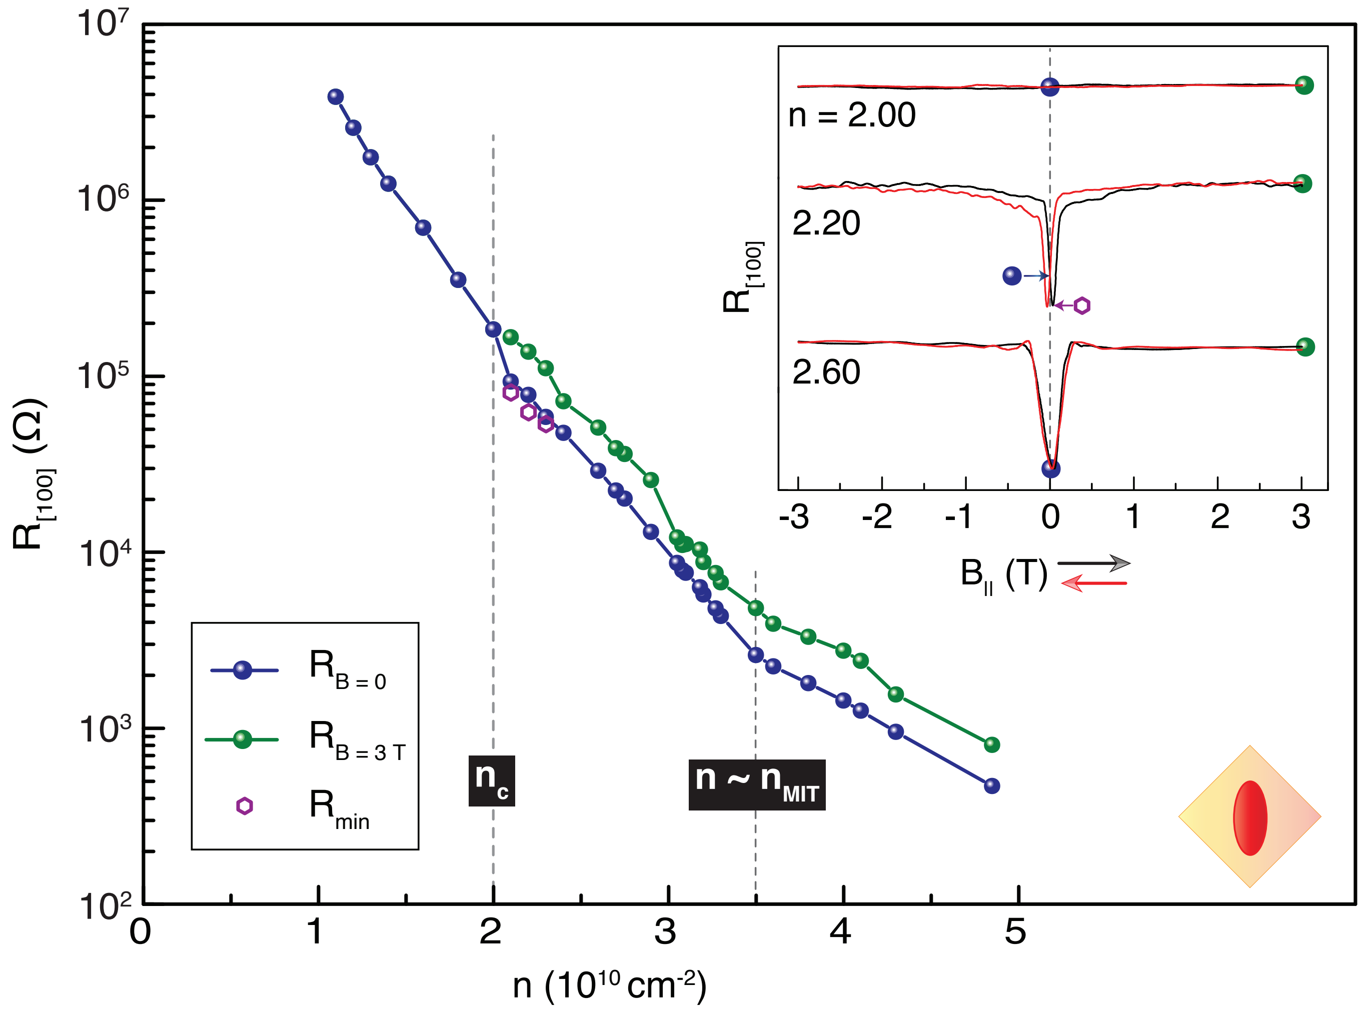


FIG. 7. Comparison between zero- and high-field values of sample resistance when the electrons are valley polarized. Plotted are the values of $R_{[100]}$ at $B_{||} = 0$ (blue circles) and 3T (green circles) as a function of electron density. Open purple symbols denote the resistance minima for the densities at which the minima are shifted from $B = 0$ due to hysteresis. The inset illustrates the field locations of the data points. At $n \leq 2.00$ (marked with a vertical line), $R_{[100]}$ is independent of $B_{||}$, leading to an overlap between blue and green points. The zero-field resistance value at $n = 2.00$ is very close to the high-field resistance value at $n = 2.10$, strongly suggesting that the 2DES is fully spin polarized at zero-field when $n = 2.00$, similar to the high-field case at $n = 2.10$. There is another sharp rise in resistance that happens near the MIT (at $n = 3.5$), also marked with a dashed vertical line.

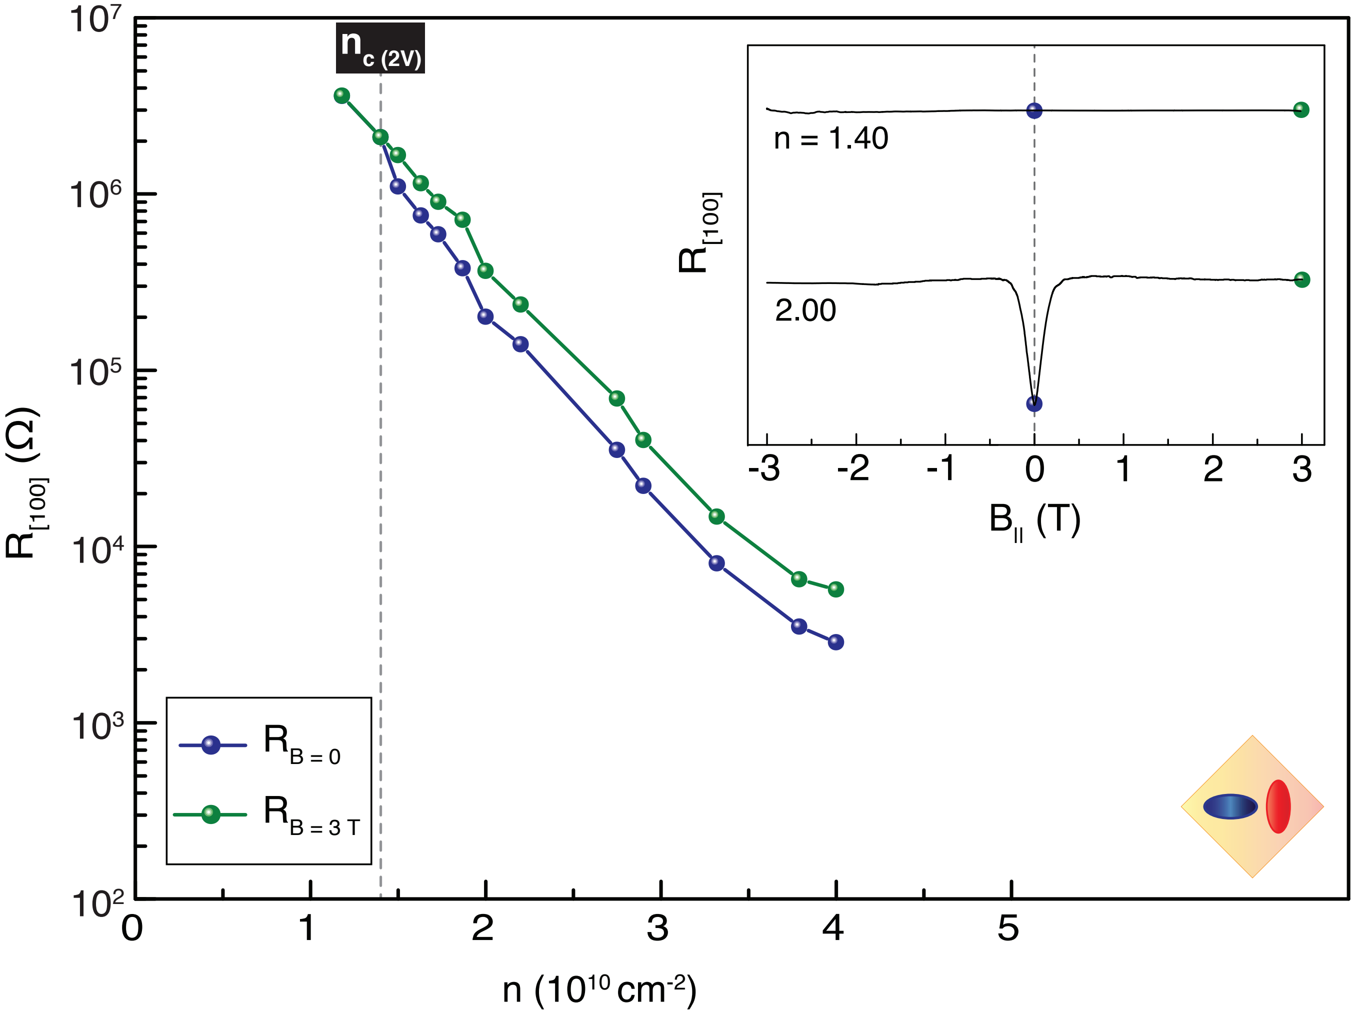


FIG. 8. Comparison between zero- and high-field values of sample resistance when the electrons occupy two degenerate valleys. Sample resistance, $R_{[100]}$ is shown against electron density; blue and green circles represent the data points at $B = 0$ and 3T, respectively. The inset shows the field positions of the two types of points. $R_{[100]}$ becomes independent of $B_{||}$ when $n \leq 1.40$ (marked with a vertical line), leading to an overlap between blue and green points. The zero-field resistance value at $n = 1.40$ approaches the high-field resistance value at $n = 1.50$, supporting our conclusion of a full-spin-polarization transition at $n = 1.40$ when the two valleys are degenerate.

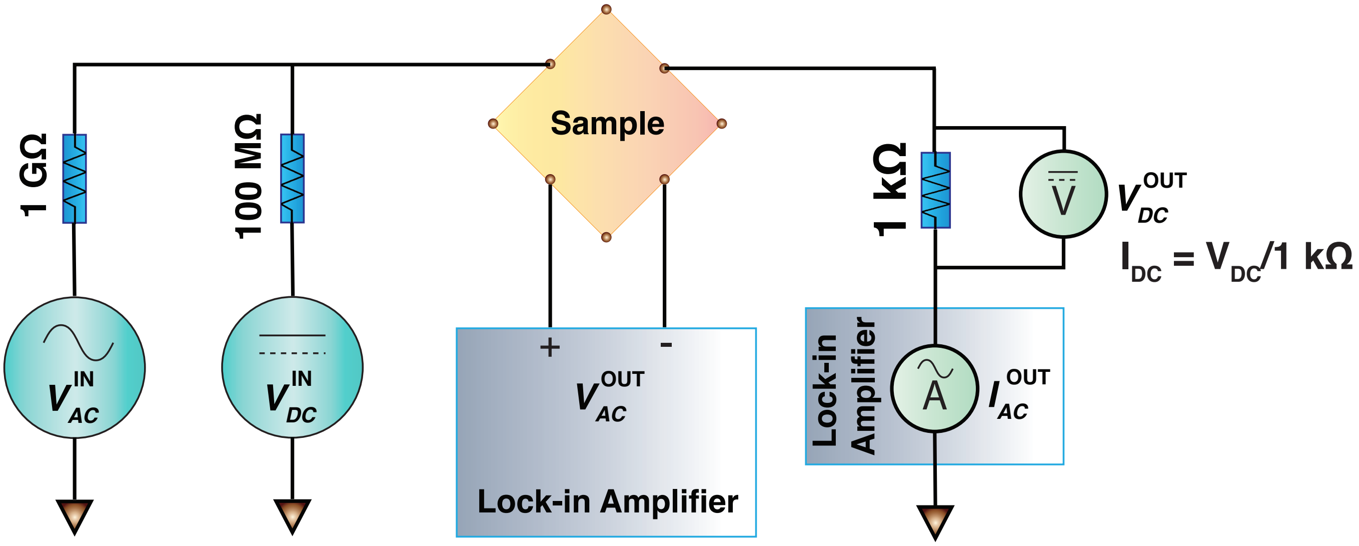


FIG. 9. Experimental setup for measuring differential resistance as a function of DC bias, showing the current injection and voltage leads used to measure both DC and AC quantities in order to obtain the $dV/dI$ vs. $I_{DC}$ plots.

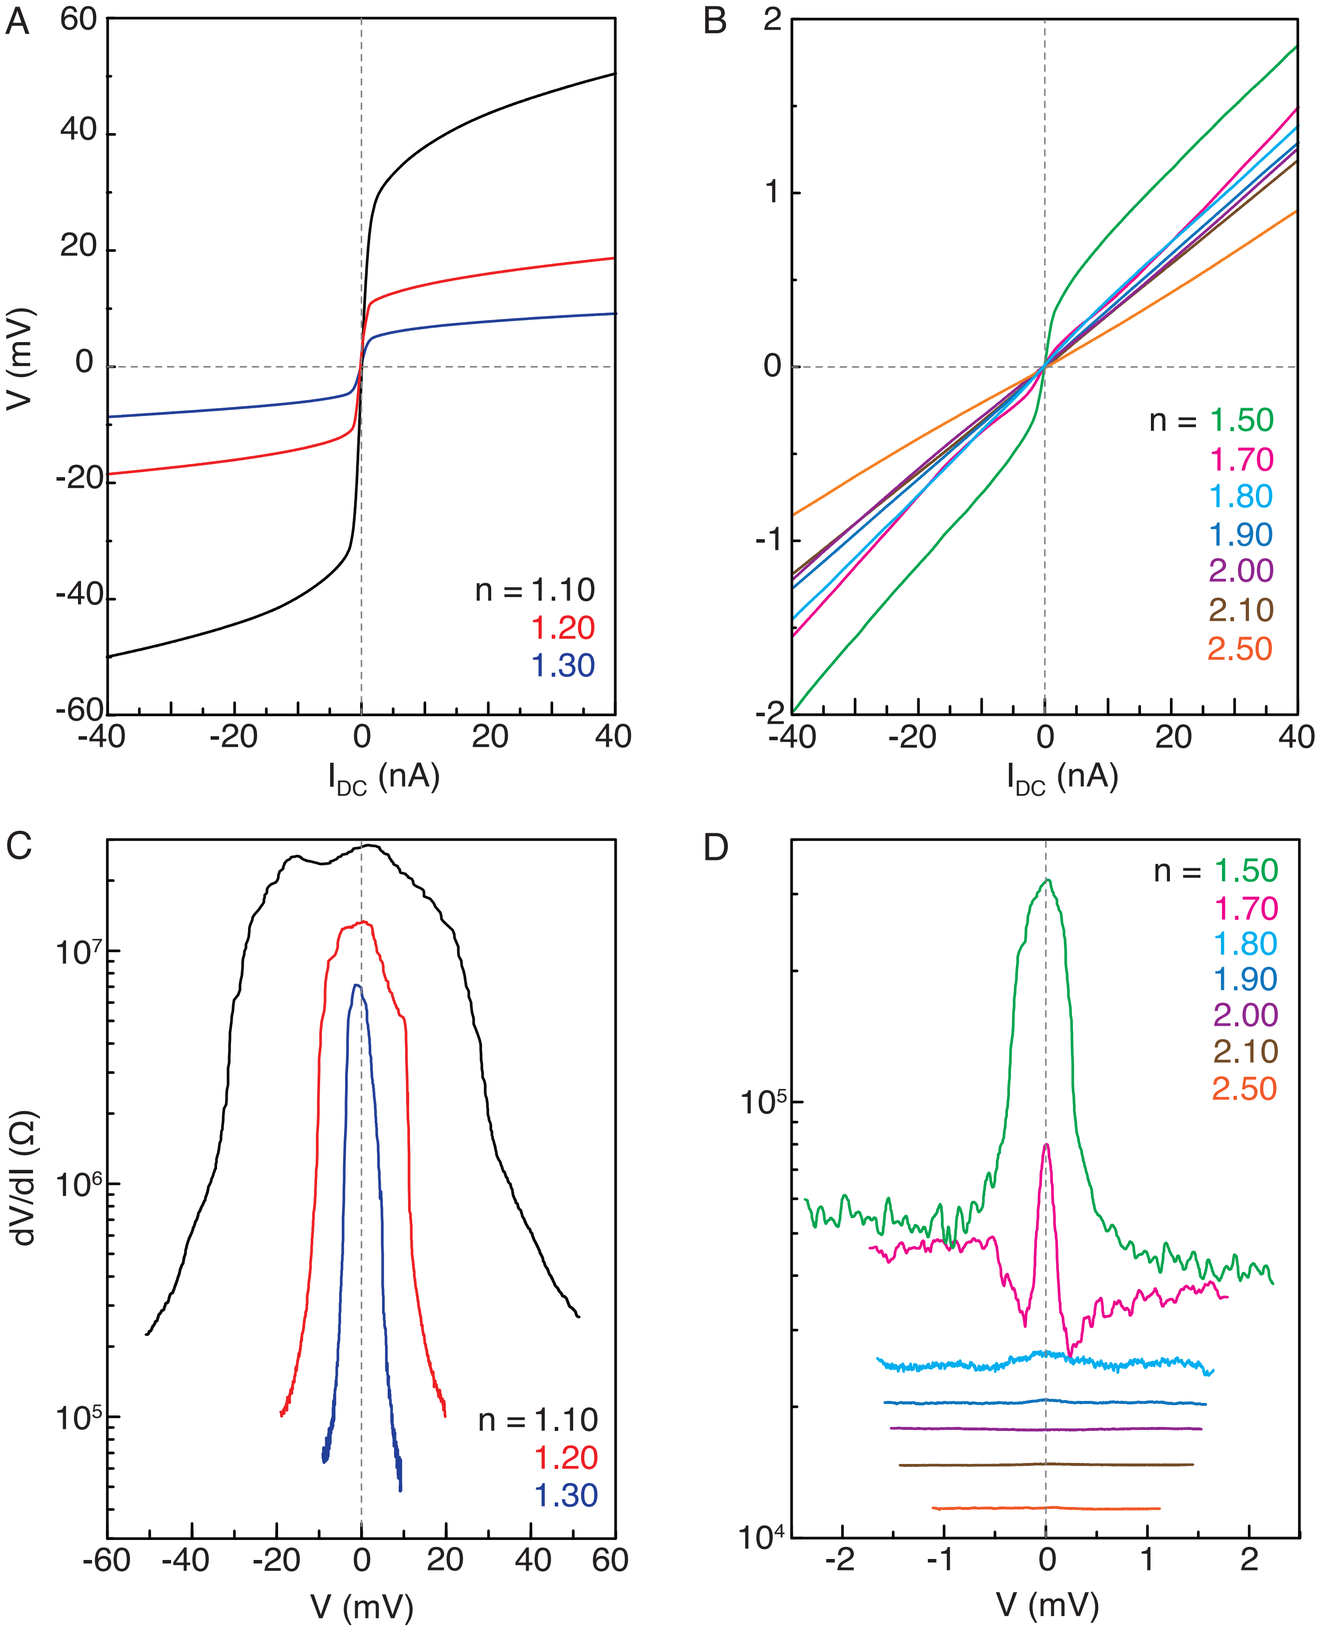


FIG. 10. Density dependence of the non-linear $I$-$V$ characteristics at $T = 0.30$ K. ($A$), ($B$) $I$-$V$ characteristics of the sample at different densities, exhibiting strong non-linearity at very low densities. ($C$), ($D$) $dV/dI$ plotted against the voltage drop along the sample. The threshold voltage is very large (about 20 mV) at $n = 1.10$, and drops significantly (to a small fraction of 1 mV) as the density is raised to $n = 1.70$ before the non-linearity disappears around $n = 1.80$. All the data are taken along the [100] direction, and only the [010] valley is occupied.

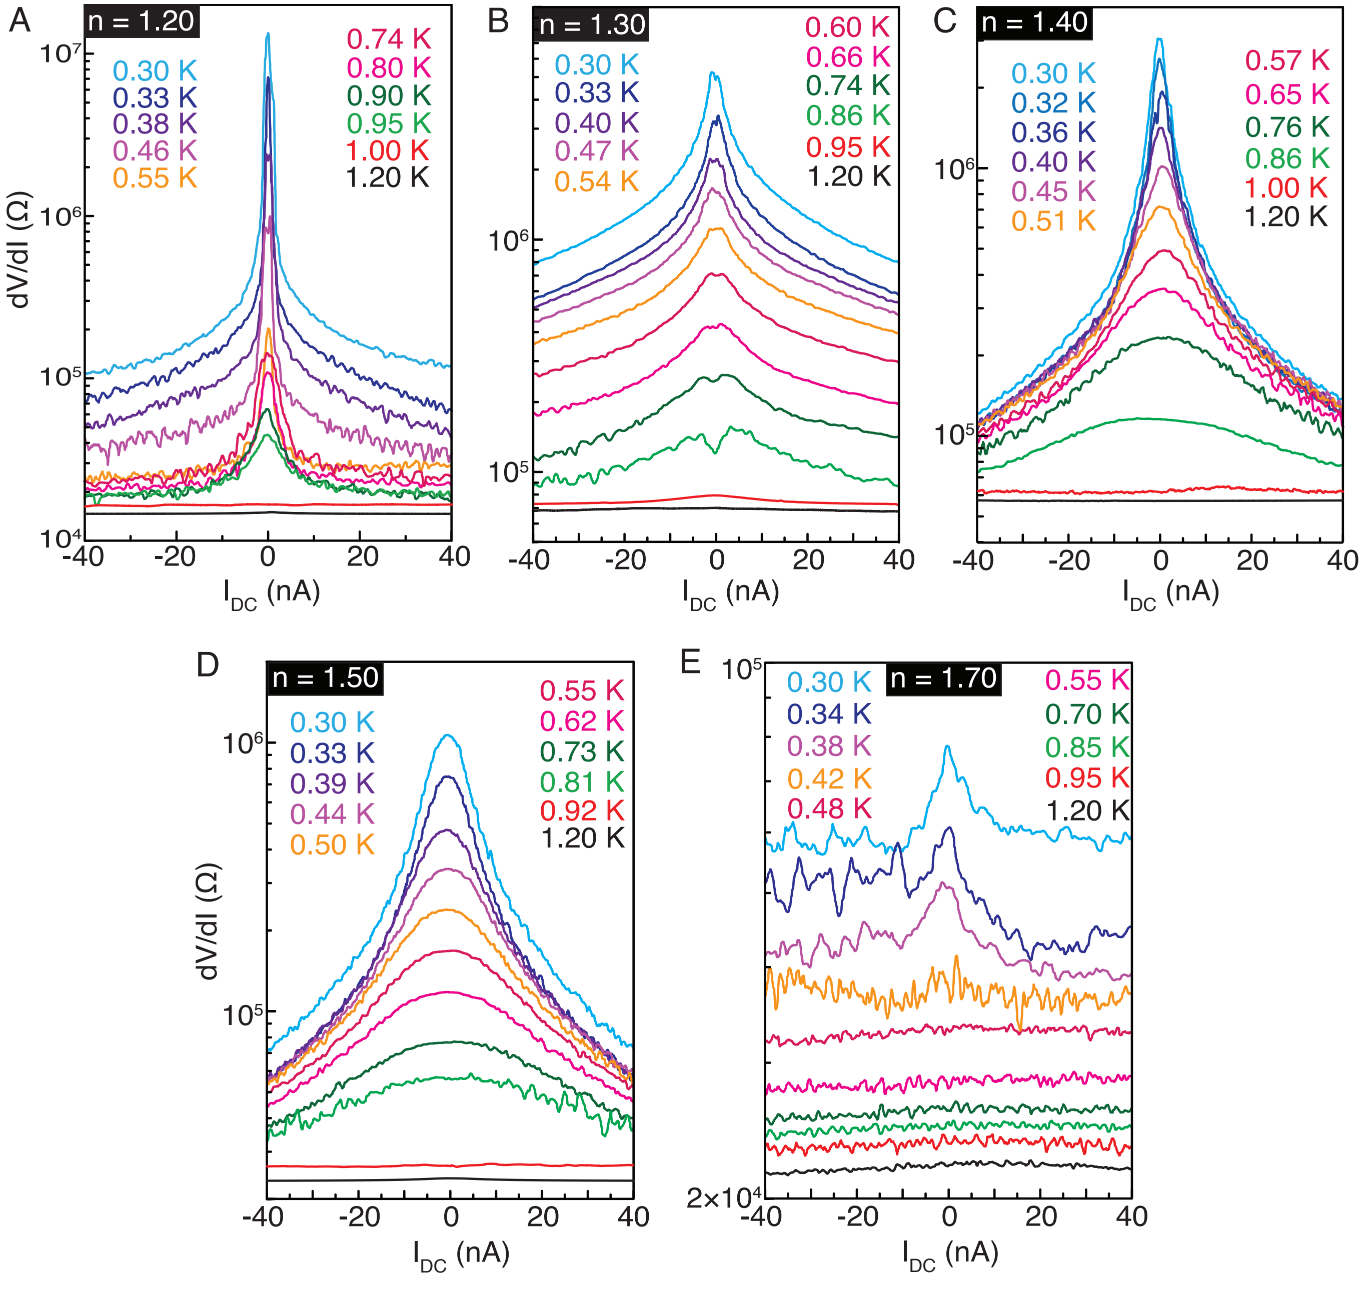


FIG. 11. Temperature dependence of $dV/dI$ measured at densities ($A$) $n = 1.20$, ($B$) 1.30, ($C$) 1.40, ($D$) 1.50, and ($E$) 1.70 along [010] direction, plotted against the DC bias current. All the electrons occupy the [010] valley. The temperature below which $dV/dI$ shows non-linearity is smaller at higher densities, implying a reduction in the melting temperature of the Wigner solid.

[1] E. P. De Poortere, Y. P. Shkolnikov, E. Tutuc, S. J. Papadakis, M. Shayegan, Enhanced electron mobility and high order fractional quantum Hall states in AlAs quantum wells. *Appl. Phys. Lett.* **80**, 1583 - 1585 (2002).

[2] M. Shayegan, E. P. De Poortere, O. Gunawan, Y. P. Shkolnikov, E. Tutuc, K. Vakili, Two-dimensional electrons occupying multiple valleys in AlAs. *Phys. Stat. Sol. (b)* **243**, 3629 - 3642 (2006).

[3] Y. J. Chung, K. A. Villegas Rosales, H. Deng, K. W. Baldwin, K. W. West, M. Shayegan, L. N. Pfeiffer, Multivalley two-dimensional electron system in an AlAs quantum well with mobility exceeding $2 \times 10^6$ $cm^2/Vs$. *Phys. Rev. Materials* **2**, 071001(R) (2018).

[4] M. Shayegan, K. Karrai, Y. P. Shkolnikov, K. Vakili, E. P. De Poortere, S. Manus, Low-temperature, in situ tunable, uniaxial stress measurements in semiconductors using a piezoelectric actuator. *Appl. Phys. Lett.* **83**, 5235 - 5237 (2003).

[5] Y. P. Shkolnikov, K. Vakili, E. P. De Poortere, M. Shayegan, Giant low-temperature piezoresistance effect in AlAs two-dimensional electrons. *Appl. Phys. Lett.* **85**, 3766 - 3768 (2004).

[6] T. Gokmen, M. Padmanabhan, M. Shayegan, Transference of transport anisotropy to composite fermions. *Nat. Phys.* **6**, 621 - 624 (2010).

[7] O. Gunawan, Y. P. Shkolnikov, K. Vakili, T. Gokmen, E. P. De Poortere, M. Shayegan, Valley susceptibility of an interacting two-dimensional electron system. *Phys. Rev. Lett.* **97**, 186404 (2006).

[8] Y. P. Shkolnikov, K. Vakili, E. P. De Poortere, M. Shayegan, Dependence of Spin Susceptibility of a Two-Dimensional Electron System on the Valley Degree of Freedom. *Phys. Rev. Lett.* **92**, 246804 (2004).

[9] M. Padmanabhan, T. Gokmen, M. Shayegan, Enhancement of valley susceptibility upon complete spin polarization. *Phys. Rev. B* **78**, 161301(R) (2008).

[10] T. Gokmen, M. Padmanabhan, M. Shayegan, Contrast between spin and valley degrees of freedom. *Phys. Rev. B* **81**, 235305 (2010).

[11] M. Marchi, S. D. Palo, S. Moroni, G. Senatore, Correlation Energy and the Spin Susceptibility of the Two-Valley Two-dimensional Electron Gas. *Phys. Rev. B* **80**, 035103 (2009).

[12] N. D. Mermin, H. Wagner, Absence of Ferromagnetism or Antiferromagnetism in One- or Two-Dimensional Isotropic Heisenberg Models. *Phys. Rev. Lett.* **17**, 1133 - 1136 (1966).

[13] J. Falson, Y. Kozuka, M. Uchida, J. H. Smet, T.-H. Arima, A. Tsukazaki, M. Kawasaki, MgZnO/ZnO heterostructures with electron mobility exceeding $1 \times 10^6$ $cm^2/Vs$. *Sci. Rep.* **6**, 26598 (2016).

[14] J. Falson, M. Kawasaki, A review of the quantum Hall effects in MgZnO/ZnO heterostructures. *Rep. Prog. Phys.* **81**, 056501 (2018).

[15] J. G. Roch, G. Froehlicher, N. Leisgang, P. Makk, K. Watanabe, T. Taniguchi, R. J. Warburton, Spin-polarized electrons in monolayer $MoS_2$. *Nat. Nanotechnol.* **14**, 432 - 436 (2019).

[16] J. G. Roch, D. Miserev, G. Froehlicher, N. Leisgang, L. Sponfeldner, K. Watanabe, T. Taniguchi, J. Klinovaja, D. Loss, R. J. Warburton, First-order magnetic phase-transition of mobile electrons in monolayer $MoS_2$. *Phys. Rev. Lett.* **124**, 187602 (2020).

[17] D. Miserev, J. Klinovaja, D. Loss, Exchange intervalley scattering and magnetic phase diagram of transition metal dichalcogenide monolayers. *Phys. Rev. B* **100**, 014428 (2019).

[18] R. Pisoni, A. Kormànyos, M. Brooks, Z. Lei, P. Back, M. Eich, H. Overweg, Y. Lee, P. Rickhaus, K. Watanabe, T. Taniguchi, A. Imamoglu, G. Burkard, T. Ihn, K. Ensslin, Interactions and Magnetotransport through Spin-Valley Coupled Landau Levels in Monolayer $MoS_2$. *Phys. Rev. Lett.* **121**, 247701 (2018).

[19] G. -B. Jo, Y. -R. Lee, J. -H. Choi, C. A. Christensen, T. H. Kim, J. H. Thywissen, D. E. Pritchard, W. Ketterle, Itinerant Ferromagnetism in a Fermi Gas of Ultracold Atoms. *Science* **325**, 1521 - 1524 (2009).

[20] E. Vermeyen, C. A. R. Sá de Melo, J. Tempere, Exchange interactions and itinerant ferromagnetism in ultracold Fermi gases. *Phys. Rev. A* **98**, 023635 (2018).

[21] Md. S. Hossain, T. Zhao, S. Pu, M. A. Mueed, M. K. Ma, K. A. V. Rosales, Y. J. Chung, L. N. Pfeiffer, K. W. West, K. W. Baldwin, J. K. Jain, M. Shayegan, Bloch ferromagnetism of composite fermions. *Nat. Phys.* (2020). https://doi.org/10.1038/s41567-020-1000-z

[22] J. K. Jain, *Composite Fermions.* (Cambridge University Press, Cambridge, 2007).
